# Supplementary material for: Self-Assembly with Geometric Tiles
Source: arXiv:1104.2809 source file (2011-04-14)
Supplement: Supplementary file 1 [file appendix.tex]

\section{Appendix} Yo!
